# Supplementary material for: Transition-Aware Multi-Activity Knowledge Tracing
Source: arXiv:2301.12916 source file (2023-01-26)
Supplement: Supplementary file 1 [file 7-appendix.tex]

\begin{figure*}[!ht]
    \centering
    \subfigure[Weight matrices of forget gate for Junyi]{
    \includegraphics[width=0.99\textwidth]{figures/Junyi/model_analysis_forgate_gate_weight_normalized_fourweights.pdf}\label{fig:trainsition_weight_junyi}}
    \subfigure[Weight matrices of forget gate for MORF]{
    \includegraphics[width=0.99\textwidth]{figures/model_analysis_forgate_gate_weight_normalized_fourweights.pdf}\label{fig:trainsition_weight_morf}}
    \subfigure[Transferring matrices of forget gate between different learning resource types for MORF]{
    \includegraphics[width=0.99\textwidth]{figures/model_analysis_forgate_gate_QL_normalized.pdf}\label{fig:trainsition_QL_morf}}
    \caption{Heatmaps for weight matrices of forget gate for Junyi and MORF dataset (a) and (b). Transferring matrices of forget gate between different learning resource types for MORF dataset (c). Rectangles show the examples we give.}
    \label{fig:transition_analysis}
\end{figure*}

\begin{figure*}[!ht]
    \centering
    \subfigure[QQ of MORF]{
    \includegraphics[width=0.5\textwidth]{figures/model_analysis_forgate_gate_QQ_normalized.pdf}\label{fig:trainsition_QL_morf}}
    \subfigure[LL of MORF]{
    \includegraphics[width=0.99\textwidth]{figures/model_analysis_forgate_gate_LL_normalized.pdf}\label{fig:trainsition_QL_morf}}
    \caption{Heatmaps for weight matrices of forget gate for Junyi and MORF dataset (a) and (b). Transferring matrices of forget gate between different learning resource types for MORF dataset (c). Rectangles show the examples we give.}
    \label{fig:transition_analysis}
\end{figure*}
